# Supplementary material for: A Survey on Scenario-Based Testing for Automated Driving Systems in High-Fidelity Simulation
Source: arXiv:2112.00964 source file (2021-12-02)
Supplement: Supplementary file 1 [file 8appendix.tex]

\appendices
\section{Table of Notations} \label{ap:notations}
We provide a table of notations shown in \Cref{tab:notation_table} for all the abbreviations used in the current work.

\begin{table}[th]
    \centering
    \begin{tabular}{l|l}
        Notation & Meaning \\
    \toprule
    {ACC} & {Adaptive Cruise Control} \\
    ADAS & Advanced    Driver-Assistance System \\
    ADS & Automated Driving System \\
    {AEB} & {Automated Emergency Braking} \\
    {ALC} & {Automated Lane Centering} \\
    {ALC2} & {Automated Lane Change} \\
    {ARM} & {Autoregressive Model} \\
    BO & Bayesian Optimization\\
    CLS & Coverage and Local Search \\
    {CNN} & {Convolutional Neural Network} \\
    DAS & Driving Automation System\\
    DE & {Differential Evolution}\\
    DNN & Deep Neural Network \\
    DRL & Deep Reinforcement Learning \\
     DT & {Decision Tree}  \\
    EA & Evolutionary Algorithm \\
    {FCW} & {Forward Collision Warning} \\
    GA & Genetic Algorithm \\
    GP & {Gaussian Process} \\
    {IL} & {Imitation Learning} \\
    {IS} & {Importance Sampling} \\
    {LDW} & {Lane Departure Warning} \\
    {NPC} & {Non-Player Character} \\
    NN & {Neural Network} \\
    NPC & Non-Player Character\\
    ODD & Operational Design Domain \\
    {OEDR} & {Object and Event Detection and Response} \\
    {PP} & {Pedestrian Protection} \\
    {RL} & {Reinforcement Learning} \\
    SA & Simulated Annealing \\
    {TSR} & {Traffic Sign Recognition} \\
    TTC & Time to Collision\\
    
    \bottomrule
    \end{tabular}
    \caption{Table of Notations.\label{tab:notation_table}}
\end{table}
